# Supplementary material for: Algorithms approaching the threshold for semi-random planted clique
Source: arXiv:2212.05619 source file (2023-06-06)
Supplement: Supplementary file 1 [file appendix.tex]

\section{Appendix} \label{sec:app-quasi-poly-brute-force}

\begin{proposition}[Quasipolynomial brute force]
The following algorithm takes a graph $G$ and, in $n^{O(\log n)}$ time, outputs a list of size $\leq (n/k)(1+\delta)$ whenever $k \geq O(\sqrt{n/\delta \log n})$.
Further, if $G \sim \FK(n,k,1/2)$, then with probability at least $0.99$ over the draw of edges in $\cut(S^*)$ in $G$ the list produced by the algorithm contains $S^*$. 

\begin{enumerate}
  \item Enumerate all $c\log n$ cliques $U$ in $G$,
  \item If $U$ and its common neighbors form a $k$-clique in $G$, add it to the list, otherwise reject, 
  \item Remove every $k$-clique in the list that intersects another in the list in more than $c \log n$ vertices. 
\end{enumerate}
\end{proposition}

\begin{proof}
Condition on the event that the planted clique $S^*$ is good.
Note that if $U \subseteq S^*$, then, notice that the common neighborhood of $U$ must equal $S^*\setminus U$ (as otherwise, there is a $k$-clique that intersects $S^*$ in $\geq c \log n$ vertices).
Thus, $S^*$ is in the list.
Further, step (3) ensures that the list only contains good cliques the number of which is at most $(1+\delta)n/k$. 
\end{proof}
